# Supplementary material for: HoWDe: a validated algorithm for Home and Work location Detection
Source: arXiv:2506.20679 source file (2025-12-01)
Supplement: Supplementary file 1 [file SI_ceus_home_work_detection.pdf]

# Supplementary Information

## Establishing validated standards for home and work location detection

### Table of Contents

|              |                                                                                    |           |
|--------------|------------------------------------------------------------------------------------|-----------|
| <b>SI-1</b>  | <b>Annotation procedure for home and work labels in Dataset2</b>                   | <b>4</b>  |
| SI-1.1       | User selection . . . . .                                                           | 4         |
| SI-1.2       | Annotation dashboard interface . . . . .                                           | 4         |
| SI-1.3       | Annotation workflow and final labeling . . . . .                                   | 5         |
| <b>SI-2</b>  | <b>Stop location: from GPS points to clusters of stop events</b>                   | <b>5</b>  |
| <b>SI-3</b>  | <b>Behavioural visit profiles</b>                                                  | <b>6</b>  |
| SI-3.1       | Detailed temporal visit patterns to home and work . . . . .                        | 6         |
| SI-3.2       | Behavioral visit profiles: results for D2 . . . . .                                | 6         |
| SI-3.3       | Behavioral visit profiles: results for D2 before and during the pandemic . . . . . | 7         |
| <b>SI-4</b>  | <b>Behavioral Clusters Entropy distribution</b>                                    | <b>9</b>  |
| <b>SI-5</b>  | <b>Stratified behavioural visit profile to home and work locations</b>             | <b>10</b> |
| <b>SI-6</b>  | <b>Algorithm structure</b>                                                         | <b>11</b> |
| <b>SI-7</b>  | <b>Detailed parameters for selected configurations</b>                             | <b>14</b> |
| <b>SI-8</b>  | <b>Validation across extended configuration parameters</b>                         | <b>14</b> |
| <b>SI-9</b>  | <b>Assessing home and work accuracy level by demographic</b>                       | <b>16</b> |
| <b>SI-10</b> | <b>Case study: Regional employment rates error rates</b>                           | <b>17</b> |

### List of Figures

|      |                                                                                                                                                                                                                                                                                                                                                                                                                                                                                                                                                                                                                                                                                |   |
|------|--------------------------------------------------------------------------------------------------------------------------------------------------------------------------------------------------------------------------------------------------------------------------------------------------------------------------------------------------------------------------------------------------------------------------------------------------------------------------------------------------------------------------------------------------------------------------------------------------------------------------------------------------------------------------------|---|
| si-1 | <b>Dataset D2 annotation dashboard.</b> Schematic of the secured-access dashboard used by independent annotators to label users' home and work locations. For each anonymized user, the dashboard displayed two maps (left) showing colored stop locations alongside summary mobility statistics (right), using a consistent colour palette. Summary statistics reported the percentage of time spent at each location by hour of the day, day of the week, and week of the year (from top to bottom). Annotators could toggle individual stops on or off, dynamically updating the time distributions to enable focused exploration of specific periods or locations. . . . . | 5 |
|------|--------------------------------------------------------------------------------------------------------------------------------------------------------------------------------------------------------------------------------------------------------------------------------------------------------------------------------------------------------------------------------------------------------------------------------------------------------------------------------------------------------------------------------------------------------------------------------------------------------------------------------------------------------------------------------|---|

|       |                                                                                                                                                                                                                                                                                                                                                                                                                                                                                                                                                                                                                                                                                                                                                                                                                                                                                                                                                                                                                                                                                                                                                                                                                                                                                                                                                                                |    |
|-------|--------------------------------------------------------------------------------------------------------------------------------------------------------------------------------------------------------------------------------------------------------------------------------------------------------------------------------------------------------------------------------------------------------------------------------------------------------------------------------------------------------------------------------------------------------------------------------------------------------------------------------------------------------------------------------------------------------------------------------------------------------------------------------------------------------------------------------------------------------------------------------------------------------------------------------------------------------------------------------------------------------------------------------------------------------------------------------------------------------------------------------------------------------------------------------------------------------------------------------------------------------------------------------------------------------------------------------------------------------------------------------|----|
| si-2  | <b>Behavioural visit profiles to home and work locations in dataset D2.</b> a. Fraction of visits per hour of the day to the annotated home locations in dataset 2, for weekdays (black) and weekends (grey) across individuals. b. Fraction of visits per hour of the day to the annotated work locations in dataset 1, for weekdays and weekends. c. Hours at home (orange), other location (grey), or without data (white), per hour of the day across days with data for weekdays. The days are sorted by cluster (divided by the black vertical lines), hour of the first home visit, total time spent at home, and hours without data. d. Hours at work (blue), other location (grey), or without data (white), per hour of the day across days with data for weekdays. The days are sorted by cluster (divided by the black vertical lines), hour of the first work visit, total time spent at work, and hours without data. e. Hours at home (orange), other location (grey), or without data (white), per hour of the day across days with data for weekends. f. Hours at work (blue), other location (grey), or without data (white), per hour of the day across days with data for weekends. . . . .                                                                                                                                                                | 7  |
| si-3  | <b>Behavioural visit profiles to home and work locations in dataset D2 during the pre-pandemic period.</b> The figure shows the user's daily behavioural patterns in the period starting from January 1st, 2020 until March 10th, 2020. a. Fraction of visits per hour of the day to the annotated home locations in dataset 2, for weekdays (black) and weekends (grey) across individuals. b. Fraction of visits per hour of the day to the annotated work locations in dataset 1, for weekdays and weekends. c. Hours at home (orange), other location (grey), or without data (white), per hour of the day across days with data for weekdays. The days are sorted by cluster (divided by the black vertical lines), hour of the first home visit, total time spent at home, and hours without data. d. Hours at work (blue), other location (grey), or without data (white), per hour of the day across days with data for weekdays. The days are sorted by cluster (divided by the black vertical lines), hour of the first work visit, total time spent at work, and hours without data. e. Hours at home (orange), other location (grey), or without data (white), per hour of the day across days with data for weekends. f. Hours at work (blue), other location (grey), or without data (white), per hour of the day across days with data for weekends. . . .      | 8  |
| si-4  | <b>Behavioural visit profiles to home and work locations in dataset D2 during the 2020 pandemic period.</b> The figure shows the user's daily behavioural patterns in the period starting from March 11th, 2020 until the end of the year. a. Fraction of visits per hour of the day to the annotated home locations in dataset 2, for weekdays (black) and weekends (grey) across individuals. b. Fraction of visits per hour of the day to the annotated work locations in dataset 1, for weekdays and weekends. c. Hours at home (orange), other location (grey), or without data (white), per hour of the day across days with data for weekdays. The days are sorted by cluster (divided by the black vertical lines), hour of the first home visit, total time spent at home, and hours without data. d. Hours at work (blue), other location (grey), or without data (white), per hour of the day across days with data for weekdays. The days are sorted by cluster (divided by the black vertical lines), hour of the first work visit, total time spent at work, and hours without data. e. Hours at home (orange), other location (grey), or without data (white), per hour of the day across days with data for weekends. f. Hours at work (blue), other location (grey), or without data (white), per hour of the day across days with data for weekends. . . . . | 9  |
| si-5  | <b>Stratified visit profiles to home and work locations.</b> Fraction of user-days per gender, age, urbanization, and country of residence GDP group (columns) by clusters of home weekday, home weekend, and work weekday (rows). The p-value of the chi-squared test measures differences across all clusters, with * indicating significant differences (p-value < 0.05). . . . .                                                                                                                                                                                                                                                                                                                                                                                                                                                                                                                                                                                                                                                                                                                                                                                                                                                                                                                                                                                           | 11 |
| si-6  | Home validation across <i>maximum days without data per sliding window</i> , $dn_H$ , (legend markers) and <i>minimum fraction of hours at home</i> , $hf_H$ , configurations for D1. . . . .                                                                                                                                                                                                                                                                                                                                                                                                                                                                                                                                                                                                                                                                                                                                                                                                                                                                                                                                                                                                                                                                                                                                                                                  | 14 |
| si-7  | Home validation across <i>maximum days without data per sliding window</i> , $dn_H$ , (legend markers) and <i>minimum fraction of hours at home</i> , $hf_H$ , configurations for D2. . . . .                                                                                                                                                                                                                                                                                                                                                                                                                                                                                                                                                                                                                                                                                                                                                                                                                                                                                                                                                                                                                                                                                                                                                                                  | 15 |
| si-8  | Work validation across <i>maximum days without data per sliding window</i> , $dn_W$ , (legend markers) and <i>minimum fraction of hours/days at work</i> , $hf_W$ , and $df_W$ , configurations for D1. . . . .                                                                                                                                                                                                                                                                                                                                                                                                                                                                                                                                                                                                                                                                                                                                                                                                                                                                                                                                                                                                                                                                                                                                                                | 15 |
| si-9  | Work validation across <i>maximum days without data per sliding window</i> , $dn_W$ , (legend markers) and <i>minimum fraction of hours/days at work</i> , $hf_W$ , and $df_W$ , configurations for D2. . . . .                                                                                                                                                                                                                                                                                                                                                                                                                                                                                                                                                                                                                                                                                                                                                                                                                                                                                                                                                                                                                                                                                                                                                                | 16 |
| si-10 | Home detection accuracy and fraction of not detected homes across demographics and configurations for D1. . . . .                                                                                                                                                                                                                                                                                                                                                                                                                                                                                                                                                                                                                                                                                                                                                                                                                                                                                                                                                                                                                                                                                                                                                                                                                                                              | 17 |

|       |                                                                                                                                                        |    |
|-------|--------------------------------------------------------------------------------------------------------------------------------------------------------|----|
| si-11 | Work detection accuracy and fraction of not detected homes across demographics and configurations for D1. . . . .                                      | 17 |
| si-12 | Estimating employment rate relative error by province, measured using the configuration with the minimum (left) and maximum (right) user loss. . . . . | 18 |

## List of Tables

|      |                                                                                                                                                                                                                                                                                                                                                      |    |
|------|------------------------------------------------------------------------------------------------------------------------------------------------------------------------------------------------------------------------------------------------------------------------------------------------------------------------------------------------------|----|
| si-1 | Table comparing normalized entropy for home and work profiles on weekdays and weekends across datasets D1 and D2. Entropy is computed for both cluster-based and randomly assigned labels, highlighting differences in profile stability. Reported values show the average and standard error of the mean computed across all users in each dataset. | 10 |
| si-2 | Configuration parameters for home detection. . . . .                                                                                                                                                                                                                                                                                                 | 14 |
| si-3 | Configuration parameters for work detection. . . . .                                                                                                                                                                                                                                                                                                 | 14 |

## SI-1 Annotation procedure for home and work labels in Dataset2

While D1 ground truth data consists of self-reported obfuscated GPS points, D2 ground truth is built leveraging insights from multiple and independent experts. This section describes the details of the procedure adopted to construct D2 ground truth.

### SI-1.1 User selection

Dataset D2 consist of 500 unique users GPS trajectories. Users were selected in a two step procedure. First, we processed stop locations and filtered uses whit a minimum level of activity consisting of at least one stop on at least 20% of days in the period before the COVID-19 pandemic declaration and of at least one stop on at least 20% of days over the entire 2020 data period. Second, we run a standard home location labelling step to estimate each users' wealth (see Fraiberger et al. [1] and Lucchini et al. [2]). Then, for each country among Brazil, Colombia, Indonesia, Mexico, and the Philippines, we sampled 100 users, 34 living in a low-wealth neighbourhood, 33 in medium-wealth neighbourhood, and 33 in high-wealth neighbourhood. This was done to reduce potential biases introduced by the minimum activity requirements in the socio-economic representativeness of the D2 ground truth data.

### SI-1.2 Annotation dashboard interface

All users' stop location sequences were then summarized and presented in a private (secured-access), navigable dashboard displaying aggregated stop-level information for single users in various formats. Only internal World Bank personnel who had explicitly signed the Data Partnership Agreement for accessing the Veraset Movements data, in the framework of the World Bank "Monitoring COVID-19 policy response through human mobility data" project, were granted access to the private dashboard. Among these people, three designated individuals were requested to perform an annotation task looking for users' home and work locations. We refer to these three individuals as 'independent annotators'.

Figure si-1 shows the structure of the dashboard that was created and made available to the independent annotators for home and work location labelling purposes. Data presented in Figure si-1 are synthetically generated data points with the sole intent of providing a more detailed understanding of the annotation procedure. The dashboard presented mobility information of one anonymised user at a time. Each coloured point on both maps (left panels) represents a user stop location. Top left panel in Figure si-1 presents an OpenStreetMap (OSM) map version including OSM Point of Interests (POIs). Bottom left panel in Figure si-1 reports a GoogleMap map version with GooglePlaces POIs and with a button to toggle satellite imagery on. Stop locations were mapped to allow annotators to easily navigate the geographical space and to better explore and inspect the geographical and land-use features of the surroundings each individual explored throughout 2020. The same colouring palette used in the maps was applied to report summary statistics about daily (hour of the day), weekly (day of the week), and yearly (week of the year) individual mobility patterns. At each time bin, the percentage of time spent at a certain location over a day, week, and year, respectively, was reported. Annotators could toggle single stops on and off. Removing one stop would result in the re-computation of the percentages of time spent in the selected locations. This was designed to simplify the process of annotators progressively exploring different stops and to facilitate focusing on specific periods or stops.

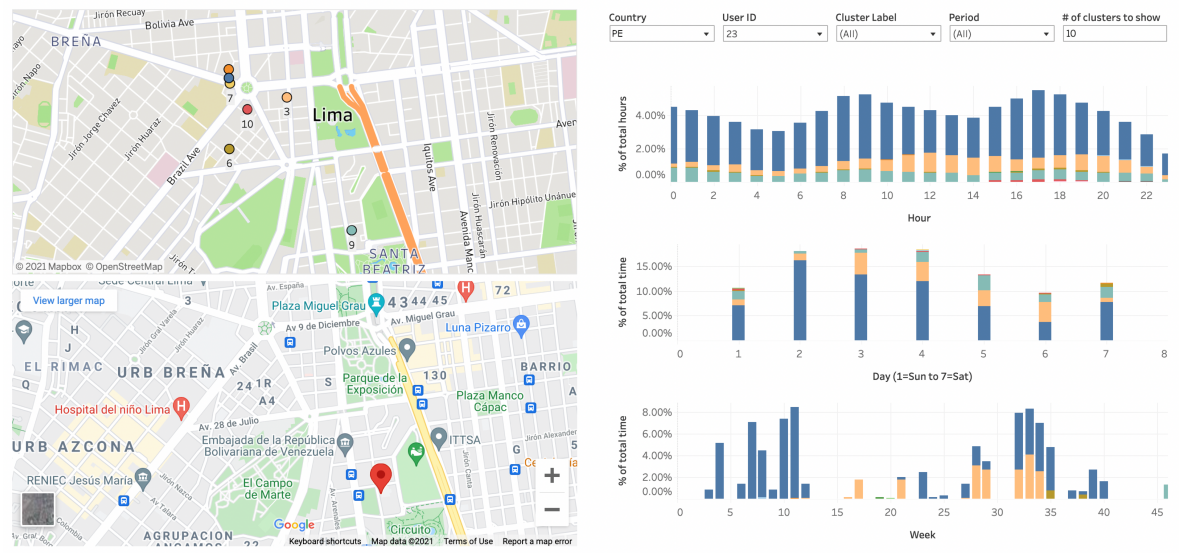

Figure si-1: **Dataset D2 annotation dashboard**. Schematic of the secured-access dashboard used by independent annotators to label users’ home and work locations. For each anonymized user, the dashboard displayed two maps (left) showing colored stop locations alongside summary mobility statistics (right), using a consistent colour palette. Summary statistics reported the percentage of time spent at each location by hour of the day, day of the week, and week of the year (from top to bottom). Annotators could toggle individual stops on or off, dynamically updating the time distributions to enable focused exploration of specific periods or locations.

### SI-1.3 Annotation workflow and final labeling

The procedure followed to obtain the final set of home and work labels is the following:

- Two independent annotators were provided with a set of identical users. For each user, one at the time, annotators were asked to identify plausible home and work location.
- Annotators were allowed to identify multiple home location for each user as well as multiple work locations.
- Responses from the two annotator were collated and compared to identify ties. Ties were then submitted to a third independent annotator for them to decide on whether the stop location that resulted as a tie was either a Home, a Work, or a different location based on the options the previous two annotators selected.
- Tie breaker results were then recombined with those labelled stop locations for which no tie occurred. This resulted in the final set of 500 user labelled stop locations.

## SI-2 Stop location: from GPS points to clusters of stop events

GPS analytics often involve the use of clustering techniques to aggregate raw GPS information into more solid structures called “stop-locations”. This is most often done in a two-step processing [3, 2]: i) spatiotemporal clustering consequent GPS point into, so-called, “stop-events”, and subsequently ii) by clustering spatially close sets of stop-events at the individual level into “stop-location” which more robustly identify as the same location those places which an individual might be visiting multiple times over the study period: both steps in this work are performed following the Infostop GPS-processing pipeline [4].

The specific parameters used for the processing differ from D1 to D2 as different types of data were involved. The main parameters involved in the stop location computations are:  $r_1$ , handling the maximum distance between two-consecutive points in a raw GPS trajectory to label them as stationary;  $r_2$ , handling the maximum distance between stationary points to form an edge, all stationary points

within range are connected and the resulting network is processed using the Infomap [5] clustering algorithm. Alternatively to the map equation for D2 we used the DBSCAN clustering algorithm which also requires a radius parameter,  $\epsilon$  (see DBSCAN method [6]). For **r1** we used respectively 30 meters in D1 and 50 meters in D2. For **r2** we used respectively 30 meters in D1 and 25 meters ( $\epsilon = 25/6371000$ ) in D2. Infostop has additional parameters to control for the shortest stop duration that can constitute a stop (**min\_staying\_time**, 10 minutes for D1 and 5 minutes for D2), the longest duration that can constitute a stop (**max\_time\_between**, 24 hours for D1 and 60 minutes for D2), and the minimum size, in terms of GPS points, a stop should be made of to be considered as stationary (**min\_size**, 2 GPS points for D1 and 2 GPS points for D2).

## SI-3 Behavioural visit profiles

### SI-3.1 Detailed temporal visit patterns to home and work

In Section *Unveiling Temporal Patterns of Home-Work Visits*, we observed a consistent pattern where home visits peak between midnight and 6 AM, while work visits are most frequent during typical business hours (9 AM–4 PM). In this section, we quantify the probabilities of being at home or work within these time ranges.

Averaging across all individuals in dataset D1, we find that during weekday nights,  $75.05\% \pm 0.60\%$  of each individual’s visits are at home. In D2, this percentage is higher,  $94.4\% \pm 0.4\%$ , due to the COVID-19 pandemic containment policies in place during most of the period covered by the data (see Sec. SI SI-3.3).

On weekends,  $69.03\% \pm 0.95\%$  of night visits occur at home (D2:  $92.1\% \pm 0.8\%$ ). In D1, home presence peaks from 1 AM to 7 AM ( $69.14\% \pm 0.94\%$ ), showing a one-hour lag compared to weekdays, while D2 remains unchanged. Beyond these hours, home probability drops sharply during business hours (9 AM–4 PM), especially on weekdays

Our analysis suggests that home detection can reliably focus on night hours without distinguishing between weekdays and weekends, as done in Atlas and Time-Geo [7, 8]). However, work detection follows a typical business hour pattern, with  $45.2\% \pm 1.2\%$  of visits occurring at the designated work location on weekdays between 9 AM and 4 PM (D2:  $35.8\% \pm 1.0\%$ ).

Outside this window or on weekends, the likelihood of being at work is minimal, around 10%. Specifically, for D1, work presence drops to  $9.5\% \pm 0.8$  on weekdays outside business hours and  $11.3\% \pm 0.9$  on weekends, while for D2, it declines to  $8.8\% \pm 0.9$  and to  $5.4\% \pm 0.6$ , respectively.

Thus, for robust home and work detection, nighttime hours (weekdays and weekends) should be prioritized for home identification, while work detection should focus on business hours during weekdays.

### SI-3.2 Behavioral visit profiles: results for D2

Here, we present the results for dataset D2 across all days. Figure si-2a,b) shows the fraction of individuals, from dataset D2, visiting on a specific random day their home, a), and work, b), location at a specific hour of the day. Black circles show the fraction of users visiting home and work during weekdays while grey crosses show the fraction during weekends. Figure si-2.c-d) reports the disaggregated visit patterns for a single “user-day” pair. In particular, it reveals that most of users’ daily patterns can be grouped into a few profiles based on their home and work visit patterns. Coloured regions (orange for home, and blue for work) show the hours of the day spent at home (Fig si-2.c,e) for weekdays and weekends respectively) and those spent at work (Fig si-2.d,f) for weekdays and weekends respectively) clustered into three different behavioural groups. Grey-coloured areas report visits to non-home locations in Figure si-2.c,e) and non-work locations in Figure si-2.d,f). Missing data are reported in white. Similar patterns as those found for D1 are found also in D2. In particular, hourly patterns show the same regularities for home and work visits, with home visits showing the highest probability in the period from midnight to 6 am and work visits in the period from 9 am to 4 pm.

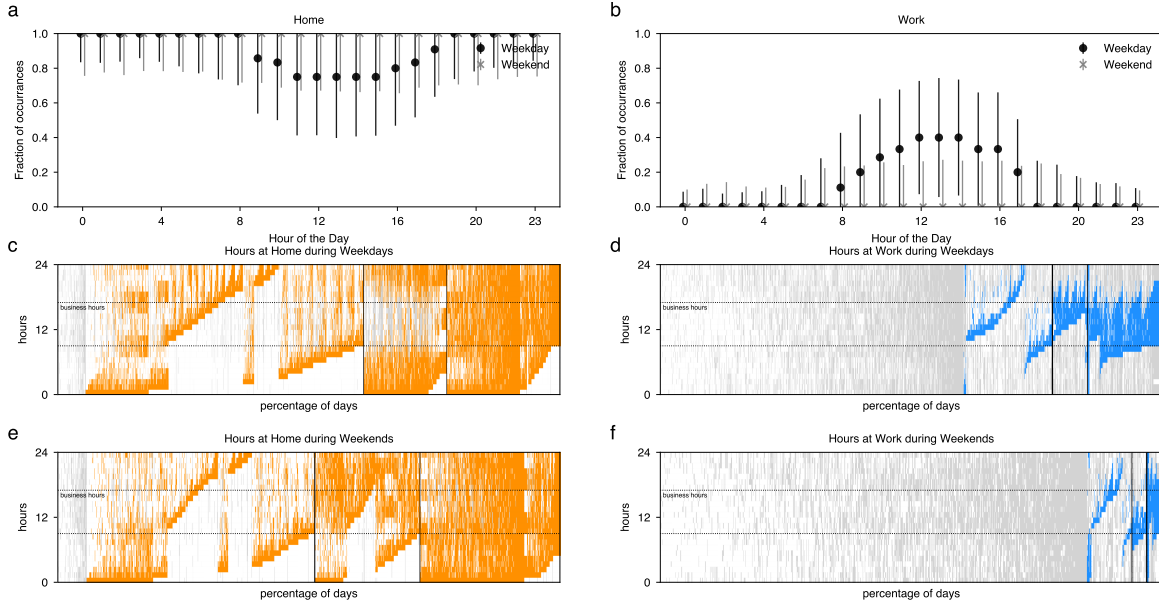

Figure si-2: **Behavioural visit profiles to home and work locations in dataset D2.** a. Fraction of visits per hour of the day to the annotated home locations in dataset 2, for weekdays (black) and weekends (grey) across individuals. b. Fraction of visits per hour of the day to the annotated work locations in dataset 1, for weekdays and weekends. c. Hours at home (orange), other location (grey), or without data (white), per hour of the day across days with data for weekdays. The days are sorted by cluster (divided by the black vertical lines), hour of the first home visit, total time spent at home, and hours without data. d. Hours at work (blue), other location (grey), or without data (white), per hour of the day across days with data for weekdays. The days are sorted by cluster (divided by the black vertical lines), hour of the first work visit, total time spent at work, and hours without data. e. Hours at home (orange), other location (grey), or without data (white), per hour of the day across days with data for weekends. f. Hours at work (blue), other location (grey), or without data (white), per hour of the day across days with data for weekends.

### SI-3.3 Behavioral visit profiles: results for D2 before and during the pandemic

Using the same procedure as in the previous section, here, we specialise the analysis to two different situations: i) in Figure si-3 we report home and work visit patterns in the period before the COVID-19 pandemic declaration. Similarly, in Figure si-4 we focus only on visit patterns after the COVID-19 epidemic was declared a pandemic by the WHO [9], on March 11th, 2020. Significant differences are found with work visitation patterns facing a three-fold contraction. Weekday-weekend differences are maintained, showing an even greater reduction in work visits. Specifically, we find that, while the highest probability of visiting workplaces occurs at similar times before and during the pandemic, the percentage of days in which users visit their workplace faced a 3.4 fold reduction (from 24.27% before the pandemic declaration to 7.21% during the pandemic). Weekend behavior shifts notably, with fewer workplace visits and more home visits during business hours. Interestingly, while the workplace visits dropped 3.4-fold during the pandemic, their timing remained unchanged.

Moreover, we also detect significant changes in home visitation patterns, with the reduction being mainly driven by reduced data quality (potentially due to reduced usage of mobile phone mobility-related applications) and patterns that get more similar to pre-pandemic “weekend” patterns.

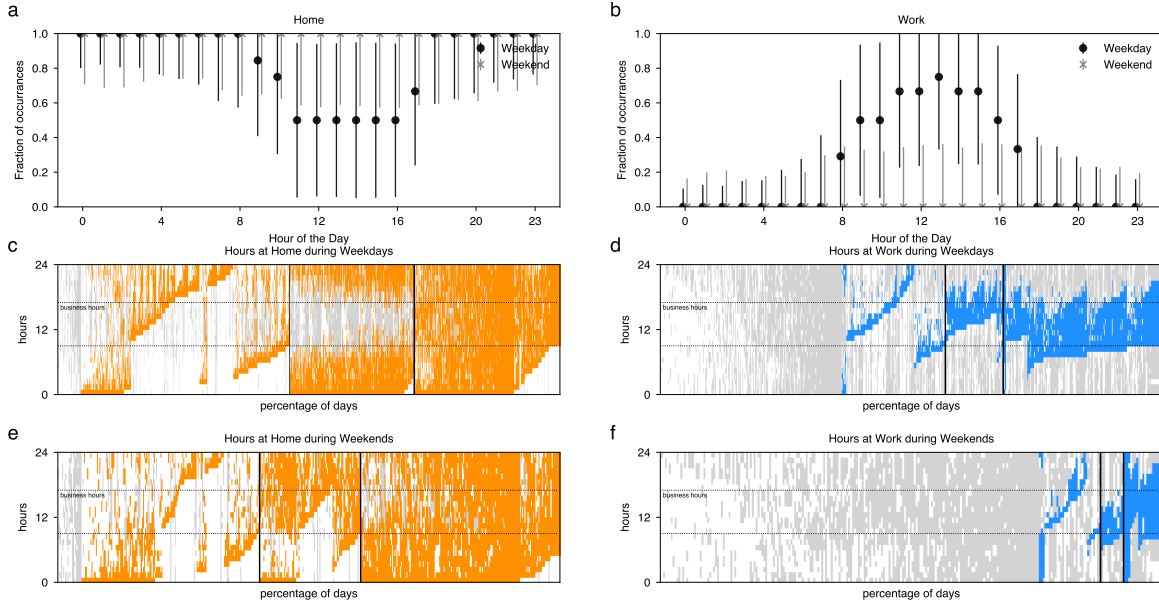

Figure si-3: **Behavioural visit profiles to home and work locations in dataset D2 during the pre-pandemic period.** The figure shows the user's daily behavioural patterns in the period starting from January 1st, 2020 until March 10th, 2020. a. Fraction of visits per hour of the day to the annotated home locations in dataset 2, for weekdays (black) and weekends (grey) across individuals. b. Fraction of visits per hour of the day to the annotated work locations in dataset 1, for weekdays and weekends. c. Hours at home (orange), other location (grey), or without data (white), per hour of the day across days with data for weekdays. The days are sorted by cluster (divided by the black vertical lines), hour of the first home visit, total time spent at home, and hours without data. d. Hours at work (blue), other location (grey), or without data (white), per hour of the day across days with data for weekdays. The days are sorted by cluster (divided by the black vertical lines), hour of the first work visit, total time spent at work, and hours without data. e. Hours at home (orange), other location (grey), or without data (white), per hour of the day across days with data for weekends. f. Hours at work (blue), other location (grey), or without data (white), per hour of the day across days with data for weekends.

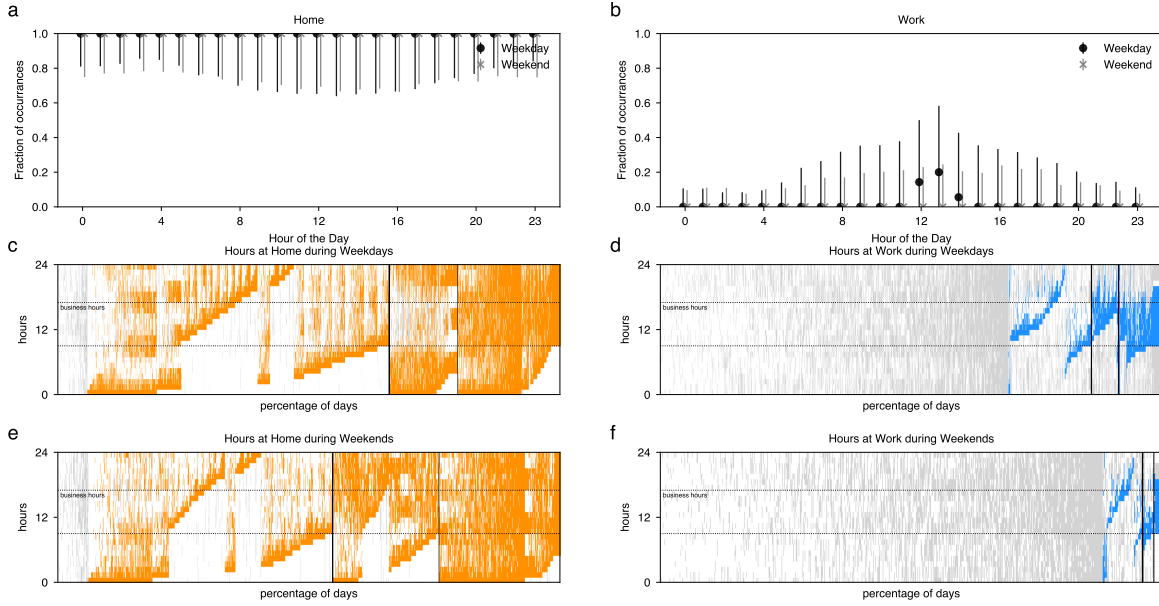

Figure si-4: **Behavioural visit profiles to home and work locations in dataset D2 during the 2020 pandemic period.** The figure shows the user’s daily behavioural patterns in the period starting from March 11th, 2020 until the end of the year. a. Fraction of visits per hour of the day to the annotated home locations in dataset 2, for weekdays (black) and weekends (grey) across individuals. b. Fraction of visits per hour of the day to the annotated work locations in dataset 1, for weekdays and weekends. c. Hours at home (orange), other location (grey), or without data (white), per hour of the day across days with data for weekdays. The days are sorted by cluster (divided by the black vertical lines), hour of the first home visit, total time spent at home, and hours without data. d. Hours at work (blue), other location (grey), or without data (white), per hour of the day across days with data for weekdays. The days are sorted by cluster (divided by the black vertical lines), hour of the first work visit, total time spent at work, and hours without data. e. Hours at home (orange), other location (grey), or without data (white), per hour of the day across days with data for weekends. f. Hours at work (blue), other location (grey), or without data (white), per hour of the day across days with data for weekends.

## SI-4 Behavioral Clusters Entropy distribution

To assess whether individuals consistently visit the same cluster or exhibit varying daily profiles, we measured the Normalized Shannon Entropy (see Methods) and compared it to a randomized test, where the daily cluster assignments were shuffled at random (only keeping the observed share of days by cluster across all users).

Table si-1 shows that the normalized entropy is moderately high across all cases, ranging from 0.40 to 0.66, indicating that users exhibit diverse daily behaviors.

As expected, entropy is consistently higher in the randomized test, where cluster labels are assigned randomly. However, the differences are not large, particularly for home visits on weekends, suggesting that users’ daily behaviors are varied and not strictly governed by a single profile.

| Test         | Dataset | Normalized Entropy |                 |
|--------------|---------|--------------------|-----------------|
|              |         | Cluster Labels     | Random Labels   |
| Home weekday | D1      | $0.66 \pm 0.00$    | $0.78 \pm 0.00$ |
|              | D2      | $0.62 \pm 0.01$    | $0.75 \pm 0.01$ |
| Home weekend | D1      | $0.48 \pm 0.01$    | $0.51 \pm 0.01$ |
|              | D2      | $0.42 \pm 0.01$    | $0.50 \pm 0.01$ |
| Work weekday | D1      | $0.51 \pm 0.01$    | $0.62 \pm 0.01$ |
|              | D2      | $0.40 \pm 0.02$    | $0.47 \pm 0.02$ |

Table si-1: Table comparing normalized entropy for home and work profiles on weekdays and weekends across datasets D1 and D2. Entropy is computed for both cluster-based and randomly assigned labels, highlighting differences in profile stability. Reported values show the average and standard error of the mean computed across all users in each dataset.

## SI-5 Stratified behavioural visit profile to home and work locations

To identify if there are discrepancies across behavioral visit profiles (see section *Unveiling Temporal Patterns of Home-Work Visits*), we stratify the days by different population groups (by age, gender, urbanization, and GDP of the country of residence) (see Fig. si-5). We focus on stratifying days to capture the possible multiple profile allocations by user. Note that each user has the same representation in days (14 days with at least 12 hours of data per day, for dataset D1)

We observe significant differences in gender, age, and urbanization across home weekday clusters, as well as for gender in home weekend clusters, as confirmed by the chi-squared test. However, to determine whether focusing on nighttime activity might exclude any demographic group, we must compare the profiles of clusters that include nighttime activity (clusters 0, 2, 3, 4, and 5) with those that exclude it (cluster 1). Our analysis reveals no significant differences among population groups, with p-values of 0.84 for gender, 0.56 for age, 0.13 for urbanization, and 0.28 for GDP, confirming the nighttime choice.

Similarly, for work weekdays, we found no significant differences in gender and age, but observed variations in GDP. To assess if focusing on typical business hours might exclude any demographic group, we analyzed cluster 1 against clusters 0 and 3. This analysis confirmed the appropriateness of focusing on business hours, with p-values of 0.25 for gender, 0.87 for age, 0.054 for urbanization, and 0.49 for income, indicating no significant exclusions. However, the lower p-value observed for urbanization, combined with the known dataset D1’s bias toward urban areas and high-income countries (see Methods), may understate potential differences.

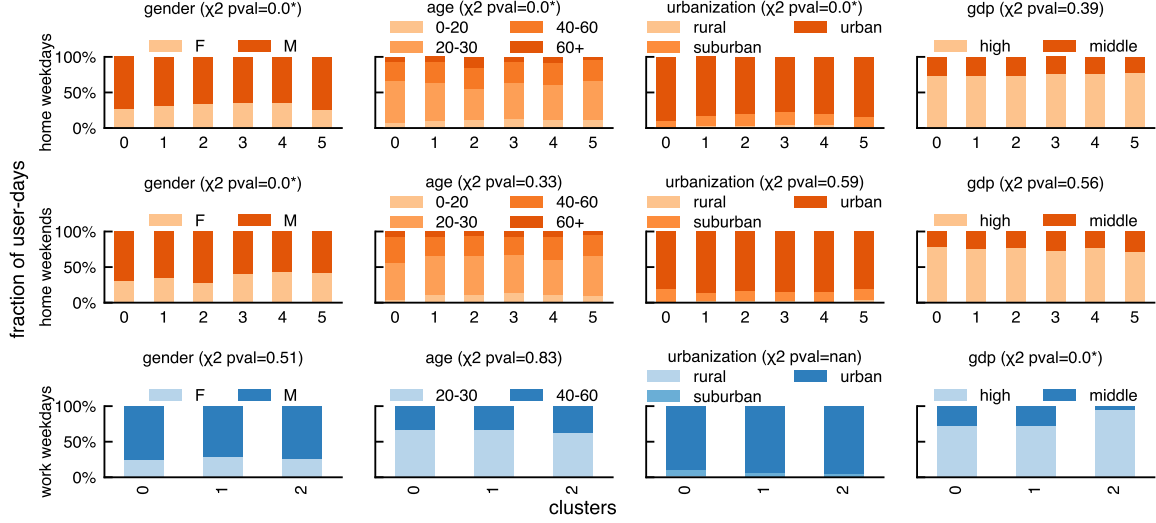

Figure si-5: **Stratified visit profiles to home and work locations.** Fraction of user-days per gender, age, urbanization, and country of residence GDP group (columns) by clusters of home weekday, home weekend, and work weekday (rows). The p-value of the chi-squared test measures differences across all clusters, with \* indicating significant differences (p-value < 0.05).

## SI-6 Algorithm structure

Here we report a complete pseudo-coded version of the algorithm presented in the manuscript. For the complete Python code we refer to [10]. We define the following quantities:

- Input time-stamped list of a user's stop events,  $S = \{T, R, E\}$ , where:
  - $T = [t_0, t_1, \dots, t_n]$  is the sequence of stop event starting timestamps,  $\forall n \in N$  with  $N$  the total number of detected stop locations;
  - $R = [r_0, r_1, \dots, r_n]$  is the sequence of stop location identifiers, note that  $r_i = r_j$  only if two stop events are clustered into the same stop location (see Sec. SI SI-2 for more details);
  - $E = [E_0, E_1, \dots, E_n]$  the sequence of stop event duration;
- Each day's hourly bins containing users' longest stop location per hour, represented as  $S_{bin} = \{D_{bin}, T_{bin}, R_{bin}\}$ , where:
  - $D_{bin} = [d_0, d_1, \dots, d_D]$  is the sequence of days where stops occur;
  - $T_{bin}^{(d)} = [t_0, t_1, \dots, t_{23}]$  is the sequence of hourly bins for each day  $d$  ( $\forall d \in D$ ), covering 24 hours;
  - $R_{bin}^{(d)} = [r_0, r_1, \dots, r_{23}]$  is the sequence of stop location identifiers visited per hourly bin on day ( $d$ ), where  $r_j^{(d)}$  corresponds to the longest stop location at hour  $j$  and day  $d$ , or None if no stop was recorded;
- $\Delta_{T_{H,W}}$  parameter fixing the length of the window used to select the consecutive days from the target day for evaluating visited locations. The window length can be set separately for home and work.
- $d_{hn}$  parameter controlling the minimum number of hours present in the *Night Hours/ Work Hours* sequence for the stops visited during the day to be considered as candidate home and work locations
- $dn_H$  parameter determining the maximum fraction of days without data per sliding window for a given day to have an estimated home location;

- 181 •  $dn_W$  parameter determining the maximum fraction of days without data per sliding window for a  
182 given day to have an estimated work location;
- 183 •  $hf_H$  parameter setting the minimum average fraction of hourly-bins (computed over the window)  
184 within the *Night Hours*-bins (considering only night hour-bins in which a user has data), required  
185 for a location to qualify as a candidate home location;
- 186 •  $hf_W$  parameter setting the minimum average fraction of hourly-bins (computed over the window)  
187 within the *Work Hours*-bins (considering only work hour-bins in which a user has data), required  
188 for a location to qualify as a candidate work location;
- 189 •  $df_W$  parameter setting the minimum fraction of days a location must be visited (among the days  
190 with data in the window) to qualify as a candidate work location;
- 191 • *NightHours* and *WorkHours* filter a user's daily stop sequences based on time constraints.  
192 *NightHours* retains only stops that end before 6 A.M. or start after 12 P.M., while *WorkHours*  
193 includes stops that start after 9 A.M. and end before 5 P.M. on working days (Monday to Friday).  
194 These can be adjusted based on the analysis needs.
- 195 •  $Window(\Delta_T, d, S_{bin})$  filters days in  $S_{bin}$  to those days within the temporal window, starting at  
196  $d - \Delta_T/2$  and terminates at  $d + \Delta_T/2$ , both included. If the 'data for prediction' parameter is  
197 selected, the window only considers past data  $d - \Delta_T$  days );
- 198 •  $HoursSeq(t_i, r_i, e_i)$  for each day with stops, aggregate stop sequences into hourly bins by splitting  
199 stops into hour intervals and assigning the stop with the longest duration per bin;
- 200 •  $HoursWithData(r_{bin}^{d\Delta})$  computes the number of hours with stop locations within a daily sequence;
- 201 •  $FracDaysW(r_{bin}^{d\Delta}, d\Delta \in D_H)$  computes the fraction of days with data within window;
- 202 •  $AvgFractVisitsHour(r_{bin}^{d\Delta})$  for each day, computes the fraction of hours each stop location was  
203 visited against the hours with data in the range studied (either night- or day-time), and averages  
204 the fraction of hours across all days in the window.
- 205 •  $FractVisitsDay(r_{bin}^{d\Delta})$  computes the fraction of days each stop location was visited, against the  
206 days with data in the window.
- 207 •  $Max\{function\}_{\forall d \in D}$  identifies the location id  $r_d$  with the highest value in *function* for the studied  
208 day  $d$
- 209 •  $First\{list\}_{\forall d \in D}$  identifies the first location id  $r_d$  in list for the studied day  $d$ . While work locations  
210 are labelled based on, first, the  $df_W$  value and, second, the  $hf_W$  value, by combining functions  
211 *First* and *Max* for work detection we enable a location to be classified as work if it meets the  
212 fraction of hours filters  $hf_W$ , even if no location satisfies the fraction of days  $df_W$ .
- 213 • *UserHasHomeS\** identifies if a given user in day  $d$  has a location previously labelled as home.

---

**Algorithm 1:** Labelling *home* and *work* locations from stop locations.

---

**Input:**  $S = \{T, R, E\}$ , where:  $T$  timestamps of user stops,  $R$  stop locations identifiers,  $E$  duration of stays at stops;  $w_H, dn_H, hf_H$ , home detection parameters;  $w_W, dn_W, hf_W, df_W$ , work detection parameters.

**Output:**  $S^* = \{T, R, E, L\}$ , where:  $L = [l_1, l_2, \dots, l_N]$  is a sequence of labels, with each  $l_i \in \{Home, Work, Other\}$ ,  $\forall i \in \{1, \dots, N\}$ , where  $N$  is the total number of detected stop locations.

```

1 # Aggregate stop sequence into hourly bins per user
  while  $i \leq N$  do
2    $S_{bin} = \{D_{bin}, T_{bin}, R_{bin}\} = HourSeq(t_i, r_i, e_i)$ 
3 end

4 # Assign labels to stop events
   $d = 0$ ;  $S^* \leftarrow \emptyset$ ;
5 while  $d \leq D$  do
6   # Define windows of  $\Delta_T$  consecutive days from  $d$  and filter to selected hours
     $S_{bin}^H = \{D_H, T_H^{(d\Delta)}, R_H^{(d\Delta)}\} = \left\{ \{d_\Delta | d_\Delta \in Window(\Delta_{T_H}, d, S_{bin})\}, \{t_j | t_j \in NightHours\}, \{r_j^{(d\Delta)} | t_j \in T_H^{(d\Delta)}\} \right\}$ 
     $S_{bin}^W = \{D_W, T_W^{(d\Delta)}, R_W^{(d\Delta)}\} = \left\{ \{d_\Delta | d_\Delta \in Window(\Delta_{T_W}, d, S_{bin})\}, \{t_j | t_j \in WorkHours\}, \{r_j^{(d\Delta)} | t_j \in T_W^{(d\Delta)}\} \right\}$ 

7   # Identify days with missing data
    forall  $d_\Delta \in D_H$  such that  $HoursWithData(r_{bin}^{(d\Delta)} \in R_H^{(d\Delta)}) \leq dhn$  do
8      $r_{bin}^{(d\Delta)} = \text{None}$ 
9   end

10  forall  $d_\Delta \in D_W$  such that  $HoursWithData(r_{bin}^{(d\Delta)} \in R_W^{(d\Delta)}) \leq dhn$  do
11     $r_{bin}^{(d\Delta)} = \text{None}$ 
12  end

13  # Home detection
    if  $FracDaysW(r_{bin}^{(d\Delta)} \in R_H^{(d\Delta)}, d_\Delta \in D_H) \geq dn_H$  and
        $AvgFractVisitsHour(r_{bin}^{(d\Delta)} \in R_H^{(d\Delta)}, d_\Delta \in D_H) \geq hf_H$  then
14     $r_d = \text{Max} \left\{ AvgFractVisitsHour(r_{bin}^{(d\Delta)} \in R_H^{(d\Delta)}, d_\Delta \in D_H) \right\}_{\forall d \in D}$ ;
15     $r_i \leftarrow r_d, \quad l_i \leftarrow H, \quad S^* \leftarrow S^* \cup \{(t_i, r_i, l_i)\}, \quad \forall t_i \in T^{(d)}$ 
16  end

17  # Work detection
    if  $FracDaysW(r_{bin}^{(d\Delta)} \in R_W^{(d\Delta)}, d_\Delta \in D_H) \geq dn_W$  and
        $AvgFractVisitsHour(r_{bin}^{(d\Delta)} \in R_W^{(d\Delta)}, d_\Delta \in D_W) \geq hf_W$  and
        $FractVisitsDay(r_{bin}^{(d\Delta)} \in R_W^{(d\Delta)}, d_\Delta \in D_W) \geq df_W$  then
18     $r_d = \text{First} \left\{ \text{Max} \{ FractVisitsDay(r_{bin}^{(d\Delta)} \in R_W^{(d\Delta)}, d_\Delta \in D_W), \text{Max} \{ AvgFractVisitsHour(r_{bin}^{(d\Delta)} \in R_W^{(d\Delta)}, d_\Delta \in D_W) \} \right\}_{\forall d \in D}$ 
19  end
20  if  $r_i \neq \emptyset$  and  $UserHasHome(S^*)$  then
21     $r_i \leftarrow r_d, \quad l_i \leftarrow W, \quad S^* \leftarrow S^* \cup \{(t_i, r_i, l_i)\}, \quad \forall l_i \neq H, \quad \forall t_i \in T^{(d)}$ 
22  end
23  else
24     $r_i \leftarrow r_d, \quad l_i \leftarrow O, \quad S^* \leftarrow S^* \cup \{(t_i, r_i, l_i)\}, \quad \forall l_i \neq H, \quad \forall t_i \in T^{(d)}$ 
25  end
26 end

```

---

## SI-7 Detailed parameters for selected configurations

Here, we report the specific configuration parameters for the selected minimum and maximum configurations. See parameter nomenclature in section SI-6.

| HoWDe Parameters | $w$ | $dhn$ | $dn_H$ | $hf_H$ |
|------------------|-----|-------|--------|--------|
| min config       | 28  | 3     | 0.7    | 0.5    |
| max config       | 28  | 3     | 0.7    | 0.9    |

Table si-2: Configuration parameters for home detection.

| HoWDe parameters | $w$ | $dhn$ | $dn_W$ | $hf_W$ | $df_W$ |
|------------------|-----|-------|--------|--------|--------|
| min config       | 42  | 3     | 0.5    | 0.4    | 0.6    |
| max config       | 42  | 3     | 0.5    | 0.6    | 0.8    |

Table si-3: Configuration parameters for work detection.

Tables si-2 and si-3 list the configuration details for dataset D1. To evaluate *HoWDe* on dataset D2, we selected a larger rolling-window width that spans the full D2 observation period ( $w = 730$ ). This choice, which tries to mirror the information available to the D2 annotators, systematically reduces the fraction of days without data in each window. Consequently, we increased  $dn_W$  to 0.7 for the D2 experiments, while keeping the other parameters identical to those used for D1.

## SI-8 Validation across extended configuration parameters

To evaluate the impact of stricter data quality requirements, we compare the accuracy and non-detection rates (see Methods) for increasing thresholds of *maximum days without data per sliding window*,  $dn_H$  and  $dn_W$  (legend markers), across different *minimum fraction of hours/days at home/work*,  $hf_H$ ,  $hf_W$ , and  $df_W$  (subplots), and varying sliding window lengths,  $\Delta_T$ .

Figures si-6 and si-7 show the effects on home detection. As observed in the main text, increasing the *minimum fraction of hours at home*,  $hf_H$ , (shown as different subplots) markedly improves accuracy but also raises the non-detection rate. In contrast, increasing the accepted *maximum fraction of days without data*,  $dn_H$ , improves user retention with only a marginal impact on accuracy, particularly in D2.

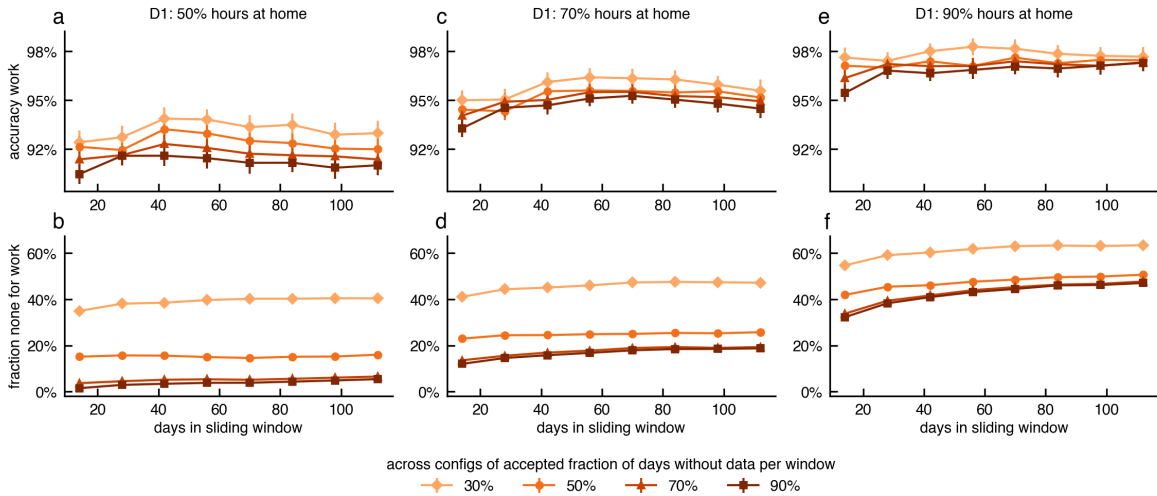

Figure si-6: Home validation across *maximum days without data per sliding window*,  $dn_H$ , (legend markers) and *minimum fraction of hours at home*,  $hf_H$ , configurations for D1.

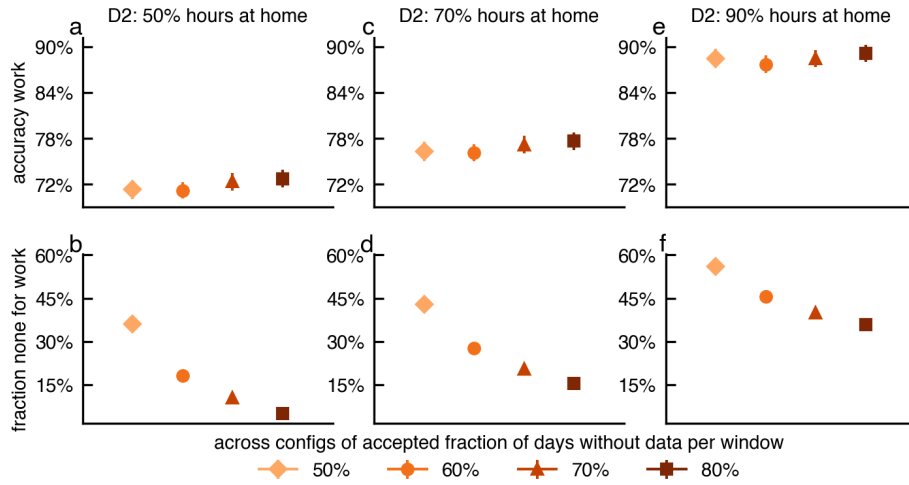

Figure si-7: Home validation across *maximum days without data per sliding window*,  $dn_H$ , (legend markers) and *minimum fraction of hours at home*,  $hf_H$ , configurations for D2.

Similar patterns emerge for work detection. As shown in Figures si-8, si-9, increasing the accepted maximum *fraction of days without data per sliding window*,  $dn_W$ , improves user retention, while accuracy remains largely unchanged for D1. In contrast, D2 shows a greater accuracy gain, likely reflecting differences in business hours data availability between datasets.

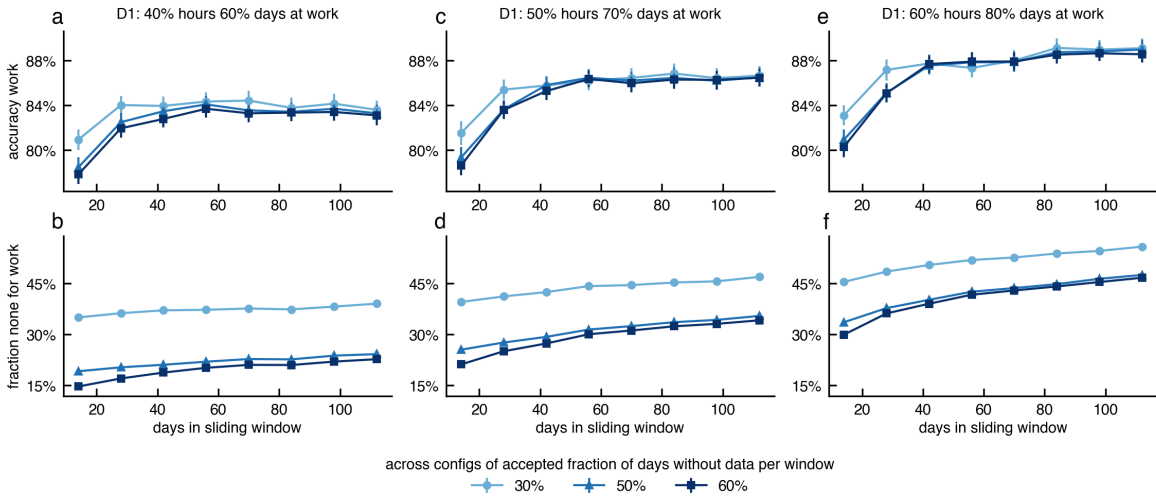

Figure si-8: Work validation across *maximum days without data per sliding window*,  $dn_W$ , (legend markers) and *minimum fraction of hours/days at work*,  $hf_W$ , and  $df_W$ , configurations for D1.

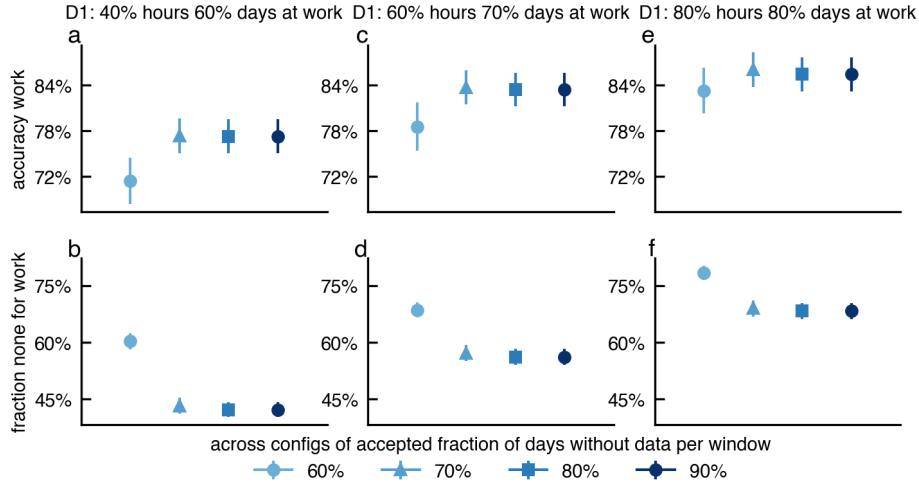

Figure si-9: Work validation across *maximum days without data per sliding window*,  $dn_W$ , (legend markers) and *minimum fraction of hours/days at work*,  $hf_W$ , and  $df_W$ , configurations for D2.

## SI-9 Assessing home and work accuracy level by demographic

To explore whether user drop affects accuracy differently across demographics, we assess the home and work detection accuracy, as well as the fraction of undetected locations, for each demographic subgroup in the "minimum" and "maximum" configurations. We present the results for subgroups comprising at least 200 users and report the associated error estimates obtained through bootstrapping.

Accuracy remains consistent across demographic groups, aligning with overall results, ranging from 90% to 99% for home detection and 77% to 89% for work detection. However, suburban areas and middle-income countries exhibit lower accuracy levels (see Figures si-10 and si-11). (see Figures si-10 and si-11).

Specifically, for suburban areas, the home detection accuracy drops by 3.39 percentage points for the minimum configuration, compared to urban areas, without a significant decline in user retention. This indicates that the drop in accuracy is smaller and not driven by a disproportionate loss of suburban users.

Individuals in middle-income countries exhibit a different pattern. The home accuracy decline is significant only in the maximum configuration, with home detection dropping by 3.31 percentage points. The effect is more pronounced for work detection, with accuracy decreasing by 9.13 and 8.06 points under the maximum and minimum configurations, respectively. Notably, these declines occur without a corresponding reduction in user retention.

This suggests two key points: first, the accuracy drop is not due to a targeted loss of users; second, the configuration that optimizes accuracy for the overall sample does not generalize to middle-income countries. Instead, the decline reflects differences in work visitation patterns.

Across other demographic groups, we find significant differences in home detection. Home accuracy drops by 1.87 points for males compared to females under the minimum configuration. For individuals aged 20–30, accuracy decreases by 2.40 and 3.60 points under the minimum and maximum configurations, respectively, relative to the 40–60 age group.

Notably, this analysis is limited to dataset D1, which is skewed toward higher-income countries and urban areas. Future research should extend validation to rural areas and low-income countries and explore intersections across demographic characteristics to better understand potential biases.

In conclusion, when choosing parameters that maximize accuracy, accuracy can vary up to 3.60% for home and 9.13% for work, across population groups. Instead, if we choose parameters that maximize user retention, accuracy varies up to 3.39% and 8.06% for home and work, respectively. These findings emphasize the importance of validating sample representativeness when applying home and work detection algorithms.

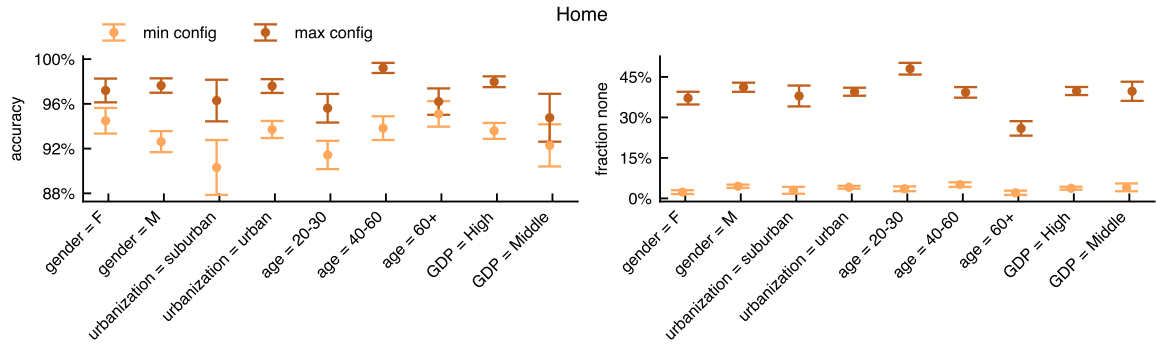

Figure si-10: Home detection accuracy and fraction of not detected homes across demographics and configurations for D1.

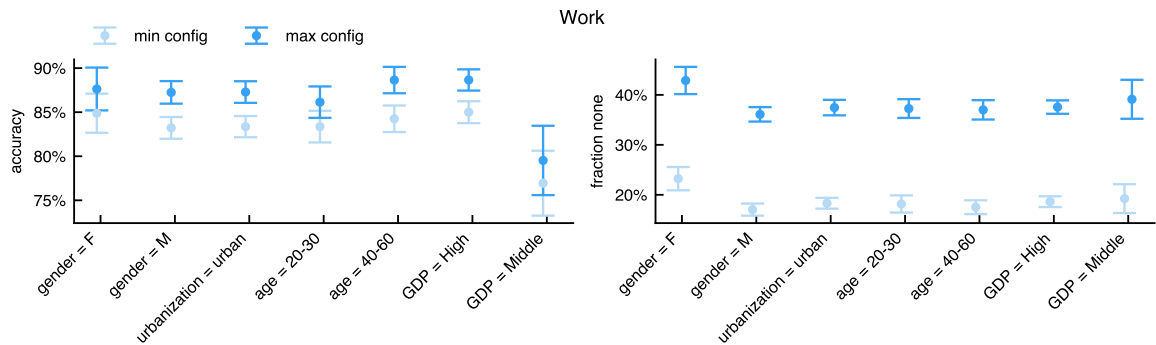

Figure si-11: Work detection accuracy and fraction of not detected homes across demographics and configurations for D1.

## SI-10 Case study: Regional employment rates error rates

Estimating employment rate relative error by province, measured using the configuration with the minimum (left) and maximum (right) user loss. Figure si-12 shows that substantially fewer regions can be estimated using the "maximum" configuration. This is mainly due to the configurations' higher thresholds on data coverage that result in a higher fraction of users for whom no work location is detected. In general, for both configurations, we find significant cross-country differences in terms of the relative error between the estimated and reported regional employment rates. Yet, across all regions and configurations, the relative error is positive, indicating that the estimated employment rates are systematically lower than the reported.

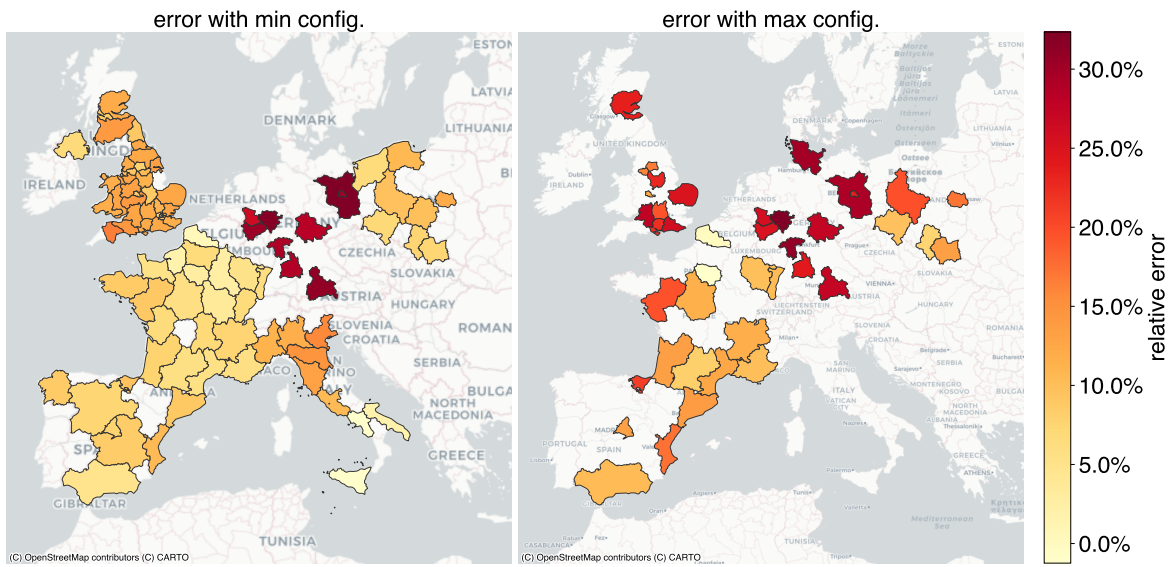

Figure si-12: Estimating employment rate relative error by province, measured using the configuration with the minimum (left) and maximum (right) user loss.

## References

- [1] Samuel P Fraiberger, Pablo Astudillo, Lorenzo Candea, Alex Chumet, Nicholas KW Jones, Maham Faisal Khan, Bruno Lepri, Nancy Lozano Gracia, Lorenzo Lucchini, Emanuele Massaro, et al. Uncovering socioeconomic gaps in mobility reduction during the covid-19 pandemic using location data. *KDD Humanitarian Mapping*, 2020.
- [2] Lorenzo Lucchini, Ollin D. Langle-Chimal, Lorenzo Candea, Lucio Melito, Alex Chumet, Aleister Montfort, Bruno Lepri, Nancy Lozano-Gracia, and Samuel P. Fraiberger. Socioeconomic disparities in mobility behavior during the covid-19 pandemic in developing countries. *EPJ Data Science*, 14(1):25, Mar 2025.
- [3] Lorenzo Lucchini, Simone Centellegher, Luca Pappalardo, Riccardo Gallotti, Filippo Privitera, Bruno Lepri, and Marco De Nadai. Living in a pandemic: changes in mobility routines, social activity and adherence to covid-19 protective measures. *Scientific reports*, 11(1):1–12, 2021.
- [4] Ulf Aslak and Laura Alessandretti. Infostop: Scalable stop-location detection in multi-user mobility data, 2020.
- [5] Daniel Edler, Anton Holmgren, and Martin Rosvall. The MapEquation software package. <https://mapequation.org>, 2024.
- [6] Martin Ester, Hans-Peter Kriegel, Jörg Sander, Xiaowei Xu, et al. A density-based algorithm for discovering clusters in large spatial databases with noise. In *kdd*, volume 96, pages 226–231, 1996.
- [7] Esteban Moro, Dan Calacci, Xiaowen Dong, and Alex Pentland. Mobility patterns are associated with experienced income segregation in large us cities. *Nature communications*, 12(1):4633, 2021.
- [8] E Moro, A Pentland, D Calacci, and X Dong. The atlas of inequality, 2021. Accessed on 2023-11-06.
- [9] WHO Director-General. Who director-general’s opening remarks at the media briefing on covid-19 - 11 march 2020. Accessed on 2024-08-06.
- [10] Silvia de Sojo, Lorenzo Lucchini, and Laura Alessandretti. Howde: a validated home and work detection algorithm. 'https://github.com/LLucchini/HowDe'.
